# Supplementary material for: Analysis and computations of a stochastic Cahn-Hilliard model for tumor growth with chemotaxis and variable mobility
Source: arXiv:2312.06288 source file (2023-12-11)
Supplement: Supplementary file 1 [file A_appendix.tex]

\appendix

\section{Elements of stochastic analysis} \label{Sec:App}
In this appendix, we collect several well-known results from stochastic analysis that we require for the existence proof in \cref{Sec:Analysis}. It is well-known that if $X$ is a Polish space (i.e., a separable completely metrizable topological space, i.e., every separable Banach space), then every probability measure on $X$ is tight. Furthermore, by Prokhorov's theorem, see \cref{Lem:Prokhorov}, a collection of probability measures on $X$ is tight if and only if it is precompact in the topology of weak convergence. 

\begin{lemma}[Gy{\"o}ngy--Krylov, cf. {\cite[Lemma 1.1]{gyongy1996existence}}] \label{Lem:GyongyKrylov}
Let $X$ be a Polish space equipped with the Borel $\sigma$-algebra. A sequence of $X$-valued random variables $(U_n)_{n\in\mathbb{N}}$ converges in probability if and only if for every sequence of joint laws of $(U_{n_k}, U_{m_k})_{k\in\mathbb{N}}$ there exists a further subsequence which converges weakly to a probability measure $\mu$ such that
\[
\mu((x, y) \in X \times X; x = y) = 1.
\]
\end{lemma}

The following theorem, due to Skorohod, links the concept of weak convergence
of a probability measure with that of almost sure convergence of random variables. Several results rely on a stochastic version of the compactness method known from the deterministic setting. Roughly speaking, the problem is the following: one constructs a sequence of approximations and to show their convergence it is necessary to establish compactness. In the presence of randomness, which is represented by the probability space, one has to be more careful, as we do not assume any topological structure and therefore the usual tools based on compact embeddings can only be applied to the time and space variable. A classical method to overcome this flaw employs Prokhorov’s and Skorokhod’s theorems.

\begin{lemma}[Prokhorov, cf. {\cite[p.37]{billingsley2013convergence}}] \label{Lem:Prokhorov}
  Let $X$ be a Polish space and $\mathcal{M}$ a collection of probability measures on $X$. Then $\mathcal{M}$ is tight if and only if it is relatively weakly compact.
\end{lemma}

\begin{lemma}[Skorokhod, cf. {\cite[Theorem 2.78]{ikeda2014stochastic}}] \label{Lem:Skorohod}
Let $X$ be a Polish space, and let $\mu_n, n \in \mathbb{N}_0$, be probability measures on $X$ such that $\mu_n$ converges weakly to $\mu_0$. Then, on some probability space, there exist $X$-valued random variables $U_n, n \in \mathbb{N}_0$, such that the law of $U_n$ is $\mu_n, n \in \mathbb{N}_0$, and $U_n(\omega) \to U_0(\omega)$ in $X$ almost surely.
\end{lemma}

\begin{lemma}[Jakubowski--Skorokhod, cf. {\cite[Theorem 2.7.1]{breit2018stochastically}}]
    \label{Lem:JakubowskiSkorokhod} Let $(X, \tau)$ be a sub-Polish space, and let $\mathcal{S}$ be the $\sigma$-field generated by $\{f_n; n \in \mathbb{N}\}$. If $(\mu_n)_{n\in\mathbb{N}}$ is a tight sequence of probability measures on $(X, \mathcal{S})$, then there exists a subsequence $(n_k)$ and $X$-valued Borel measurable random variables $(U_k)_{k\in\mathbb{N}}$ and $U$ defined on the standard probability space $([0,1], \mathcal{B}([0,1]), \mathcal{L})$ such that $\mu_{n_k}$ is the law of $U_k$, and $U_k(\omega)$ converges to $U(\omega)$ in $X$ for every $\omega \in [0, 1]$. Moreover, the law of $U$ is a Radon measure.
\end{lemma}

\begin{lemma}[cf. {\cite[Theorem 1.10.4]{wellner2013weak}}] \label{Lem:Convergence}
    Let $X_a:\Omega_a \to D$ be an arbitrary
net indexed by a nontrivial directed set, and let $X_\infty$ be Borel measurable
and separable. If $X_a \to X_\infty$, then there exists a probability space $(\widetilde \Omega, \widetilde A, \widetilde \bbP)$
and maps $\widetilde X_a:\widetilde \Omega \to D$ with $X_a \to X_\infty$ and $\bbE^*f(\widetilde X_a) = \bbE^*f(X_a)$, for every bounded $f:D\to \bbR$ and every $a$. Moreover, for $\phi_a:\widetilde \Omega \to \Omega_a$ measurable and perfect, one can choose $\widetilde X_a=X_a \circ \phi_a$ and $\bbP_a=\widetilde \bbP \circ \phi_a^{-1}$.
\end{lemma}

\begin{lemma}[Burkholder--Davis--Gundy inequality, cf. {\cite[Lemma 7.2]{da1996stochastic}}] \label{Lem:BurkholderDavisGundy}
Let $H$ be a separable Hilbert space. Let $p \in (0, \infty)$. There exists a constant $C_p > 0$ such that, for every $(\mathcal{F}_t)$-progressively measurable stochastic process $G$ satisfying $\mathbb{E} \int_0^T \left\| G(t) \right\|_{L^2(\mathcal{U}, H)}^2 \, dt <\infty,$ the following holds:
\[
\mathbb{E} \sup_{t \in[0,T]} \left\| \int_0^t G(s) \, dW(s) \right\| \leq C_p \mathbb{E} \left( \int_0^T \left\| G(s) \right\|_{L^2(\mathcal{U}, H)}^2 \, ds \right)
\]
\end{lemma}

A family $\Lambda$ is said to be compact (respectively relatively compact) if an arbitrary
sequence $(\mu_n)_n$ of elements from $\Lambda$ contains a subsequence $(\mu_{n_k})_k$ weakly convergent to a measure $\mu \in \Lambda$ (respectively to a measure $\mu$ on $(E,\scrB(E))$).

\begin{lemma}[Stochastic Gronwall, cf. {\cite[Lemma 29.1]{metivier2011semimartingales}}] \label{Lem:Gronwall}
    Let $A$ be an adapted, right-continuous, increasing, positive process defined on the stochastic interval $\left[0,\tau\right)$ and such that $\sup_{t<\tau} A_t \leq l \in \bbR^+$. Let $\Phi$ be a real-increasing, adapted process such that, for every stopping time $\sigma \leq \tau$, 
    $$\bbE(\Phi_{\sigma^{-}}) \leq K + \rho \bbE\left(\int_{\left[0,\sigma\right)} \Phi_{s^{-}} \d s_s\right),$$
    where $K$ and $\rho$ are two constants. Then
        $$\bbE(\Phi_{t^{-}}) \leq 2K \sum_{j=0}^{[2\rho l]} (2 \rho l)^j,$$
        where $[x]$ denotes the integer part of $x \geq 0$.
\end{lemma}

\begin{lemma}
    Let $W = \sum_{k=1}^\infty e_k W_k$ be a cylindrical Wiener process in a separable Hilbert space $\mathcal{U}$. Let $G$ be an $L^2(\mathcal{U}; H)$-valued stochastically integrable process, $g$ be an $H$-valued progressively measurable Bochner integrable process, and let $U(0)$ be an $\mathcal{F}_0$-measurable $H$-valued random variable. Then the process
\[
U(t) = U(0) + \int_0^t g(s) \, ds + \int_0^t G(s) \, dW(s)
\]
is well-defined.
Assume that a function $F \colon H \to \mathbb{R}$ and its derivatives $F'$, $F''$ are uniformly continuous on bounded subsets of $H$.
Then we have almost surely, for all $t \in [0,T]$,
\[\begin{aligned}
F(U(t)) &= F(U(0)) + \int_0^t \langle F'(U(s)), g(s) \rangle \, ds + \int_0^t \langle F'(U(s)), G(s) \, dW(s) \rangle_{1,t} \\ &\quad+ 2 \int_0^t \text{Tr}\left(G(s)^*F''(U(s))G(s)\right) \, ds,
\end{aligned}\]
where $\text{Tr}(A) = \sum_{k=1}^\infty \langle A e_k, e_k \rangle$ for $A$ being a bounded linear operator on $H$.
\end{lemma}

\begin{lemma}
    Assume that $U$ and $V$ are $H$-valued stochastic processes defined on the same probability space and satisfying the assumptions of Theorem 2.4.1. Assume that they admit the decompositions
\[
\begin{aligned}
U(t) &= U(0) + \int_0^t g(s) \, ds + \int_0^t G(s) \, dW(s), \quad t \in [0,T], \\
V(t) &= V(0) + \int_0^t h(s) \, ds + \int_0^t H(s) \, dW(s), \quad t \in [0,T].
\end{aligned}
\]
Then, we have
\[
\begin{aligned}
\langle U(t), V(t) \rangle &= \langle U(0), V(0) \rangle + \int_0^t \langle V(s), g(s) \rangle \, ds + \int_0^t \langle V(s), G(s) \, dW(s) \rangle \\
&\quad+ \int_0^t \langle U(s), h(s) \rangle \, ds + \int_0^t \langle U(s), H(s) \, dW(s) \rangle + \sum_{k=1}^\infty \int \langle G(s) e_k, H(s) e_k \rangle \, ds.
\end{aligned}
\]

\end{lemma}

\begin{lemma}[It\^{o}] \label{Lem:Ito}  
Assume that $U$ is a continuous $V^*$-valued stochastic process given by
\[
U(t) = U(0) + \int_0^t g(s) \, ds + \int_0^t G(s) \, dW(s), \quad t \in [0, T],
\]
where $G \in L^2(\Omega \times [0, T]; L^2(\mathcal{U}; H))$, $g \in L^2(\Omega \times [0, T]; V^*)$, and both are progressively measurable. Also, $U(0) \in L^2(\Omega; H)$ is $\mathcal{F}_0$-measurable.
If $U \in L^2(\Omega \times [0, T]; V)$, then $U$ is an $H$-valued continuous stochastic process, and
\[
\mathbb{E} \sup_{t \in [0, T]} \|U(t)\|_H^2 < \infty,
\]
and the following Itô formula holds true almost surely:
\[ \begin{aligned}
\|U(t)\|_H^2 &= \|U(0)\|_H^2 + 2\int_0^t \langle g(s), U(s) \rangle_{V^*, V} \, ds + 2\int_0^t \langle U(s), G(s) \, dW(s) \rangle_H
\\ &\quad+ \int_0^t \|G(s)\|_{L^2(\mathcal{U}; H)}^2 \, ds, \quad \text{for any } t \in [0, T].
\end{aligned} \]
\end{lemma}
